# Supplementary material for: Semantic Completeness for Correct Maintenance: A Strict Hierarchy of Typing and Inheritance
Source: arXiv:2601.14252 source file (2026-11-02)
Supplement: Supplementary file 1 [file appendix_lean.tex]

\subsection{Formalization and Verification}\label{formalization-and-verification}

The Lean formalization certifies the declared model, admissibility contract, and main theorem chain in the finite explicit setting. Mechanization therefore provides a formal check that the stated impossibility and optimality claims follow from the declared regime and that no unstated side channels are required. The appendix remains concise; the full proof artifacts are provided as a supplementary formalization release.

The detailed Lean module table is provided in supplementary material. It lists the 10 core modules with line counts, theorem counts, and purposes.

\paragraph{What is in scope in the mechanization.}
The formalization covers the abstract observer model, the information barrier, adaptive fiberwise side-information budgets, task-level sufficiency under fixed representations, helper-view fusion laws, exact product-fiber laws for factorized representations, structured axis families with derivability-aware closure, and the zero-error frontier claims stated in the main text. The structured-axis layer includes closure, exchange, equicardinality, and basis results. The converse chain, graph-confusability threshold and block-scaling results, adaptive side-information layer, and task-level laws are all represented in the cited theorem stack, including positive-distortion and learned-representation finite explicit corollaries. The Lean development works in the finite explicit setting used by the theorem statements: finite class sets, finite attribute families, and explicit profile maps or induced finite relations. It certifies the converse, block-scaling laws, adaptive fiberwise lower and upper bounds, task-level sufficiency, helper-view fusion laws, factorized product laws, the finite deterministic distortion floor, and the restricted structured-axis matroid bridge in that setting rather than the complexity of estimating $A_\pi$ from an implicit representation such as a circuit, program, or learned model. \leanmeta{\LH{L1}, \LHrng{L}{4}{5}, \LHrng{LWDC}{1}{3}, \LH{GPH13}, \LH{GPH16}, \LHrng{GPH}{18}{19}, \LH{GPH24}, \LHrng{GPH}{27}{28}, \LH{GPH30}, \LHrng{GPH}{32}{43}}

\paragraph{Claim backing in the main text.}
The main text uses inline handle tags as claim-level links into the formalization, and the automatically generated handle index records the corresponding Lean declarations. The claims-only verification pass for the current release marks 10 main-text claims with explicit proof paths, so the emphasis is on which claims are backed rather than on aggregate artifact size. \leanmeta{\LH{GPH35}}

\paragraph{What is moved to supplementary artifact.}
Implementation-specific operational details and extended code listings are included in supplementary material and are not required to follow the IT contribution in the main paper.

\subsection{Attribute-Only Formalization}\label{interface-only-formalization}

Attribute-only observation is formalized by an equivalence relation on values induced by observable query responses.

\begin{lstlisting}[style=lean]
structure InterfaceValue where
  fields : List (String * Nat)
deriving DecidableEq

def getField (obj : InterfaceValue) (name : String) : Option Nat :=
  match obj.fields.find? (fun p => p.1 == name) with
  | some p => some p.2 | none => none

def interfaceEquivalent (a b : InterfaceValue) : Prop :=
  forall name, getField a name = getField b name

def InterfaceRespecting (f : InterfaceValue -> a) : Prop :=
  forall a b, interfaceEquivalent a b -> f a = f b
\end{lstlisting}

\subsection{Corollary 6.3: Provenance Impossibility}\label{corollary-6.3-interface-only-cannot-provide-provenance}

Under attribute-only observation, provenance is constant on attribute-equivalence classes; therefore provenance cannot be recovered when distinct classes collide under the observable profile.

\begin{lstlisting}[style=lean]
theorem interface_provenance_indistinguishable
    (getProvenance : InterfaceValue -> Option DuckProvenance)
    (h_interface : InterfaceRespecting getProvenance)
    (obj1 obj2 : InterfaceValue)
    (h_equiv : interfaceEquivalent obj1 obj2) :
    getProvenance obj1 = getProvenance obj2 :=
  h_interface obj1 obj2 h_equiv
\end{lstlisting}

This is the mechanized form of the main-text impossibility statement: if an observer factors through attribute profile alone, it cannot separate equal-profile values by source/provenance.

\subsection{Abstract Model Lean Formalization}\label{abstract-model-lean-formalization}

The abstract model is formalized directly at the axis level and then connected to concrete instantiations.

\begin{lstlisting}[style=lean]
-- Axis-indexed representation
abbrev Typ (A : Finset Axis) := (a : Axis) -> a \in A -> axisType a

-- Two-axis formal setting
abbrev Typ2 := Typ ({Axis.Bases, Axis.Shape} : Finset Axis)

-- Projectors
abbrev projBases (t : Typ2) := t Axis.Bases (by simp)
abbrev projShape (t : Typ2) := t Axis.Shape (by simp)
\end{lstlisting}

The corresponding isomorphism theorem establishes that the two-axis representation is complete for in-scope observables in the formal model.

\subsection{Reproducibility}

The full Lean development is provided in supplementary material. To verify locally:
\begin{enumerate}
\item Install Lean 4 and Lake (\url{https://leanprover.github.io/}).
\item From the release package root, run:
\begin{lstlisting}[style=lean]
cd proofs
lake build
\end{lstlisting}
\item Confirm successful build with no \texttt{sorry} placeholders.
\end{enumerate}
